# Supplementary material for: Debiasing In-Sample Policy Performance for Small-Data, Large-Scale Optimization
Source: arXiv:2107.12438 source file (2022-08-02)
Supplement: Supplementary file 1 [file B_Strong_Convex_Appendix.tex]

%!TEX root = 0_main.tex
\section{Approximate Strong Convexity}

Recall that a function $f(\cdot)$ is $\gamma$-strongly convex if\footnote{This definition is equivalent to the ``usual" definition of strong convexity.} 
\begin{equation} \label{eq:StrongConvexityDefinition}
\left( \nabla f(\bx)  - \nabla f(\by) \right)^\top (\bx - \by) \geq \gamma \| \bx - \by \|^2  \quad \forall \bx, \by \in \text{Dom}(f).
\end{equation}

We next argue that the dual objective function satisfies a similar condition.  Let
\begin{align*}
	\blambda( \bZ) \in \arg \min_{\blambda \geq \bzero} \ \bm{b}^\top \blambda + \frac{1}{n} \sum_{j=1}^n [Z_j - \bA_j^\top \blambda]^+.
\end{align*}  
From G\&R that there exists a dimension-independent constant $\lambda_{\max} > 1$ such that $\| \blambda(\bZ) \|_1 \leq  \lambda_{\max}$ with probability at least $1-\exp(-Cn)$ for some dimension-independent constant $C$ (see Lemma D.3 part ii) of G\&R).

Notation and set up follows G\&R 2019.  In particular, $C_A$ is a constant such that $\| \bA_j \| \leq C_A$ for all $1 \leq j \leq n$, $m \geq 1$, the minimal eigenvalue of $\frac{1}{n} \sum_{j=1}^n \bA_j \bA_j^\top \geq \beta > 0$, and $Z_j$ are Gaussian satisfying the following conditions:
\begin{assumption}[Density Bounded]  \label{asn:BoundedDensity}  We assume throughout
	\begin{itemize}
		\item There exists $\phi_{\min} > 0$ such that the density of $Z_j$ at a point $t$ is lower-bounded by $\phi_{\min}$ for all $\abs{t} \leq C_A \lambda_{\max} + 1$ for all $j =1, \ldots, n$.
		\item There exists $\phi_{\max} > 0$ such that the density of $Z_j$ at a point $t$ is upper-bounded by $\phi_{\min}$ for all $\abs{t} \leq C_A \lambda_{\max} + 1$ for all $j=1, \ldots, n$.
	\end{itemize}
\end{assumption}
A sufficient condition for \cref{asn:BoundedDensity} is that $\nu_j$ is bounded away from $0$ and $\infty$ for all $j$,  i.e.,  $\nu_{\min} \le \nu_j \le \nu_{\max}$ for constants $\nu_{\min},\nu_{\max}$. 

Our overall strategy is to show 
\begin{enumerate}
	\item The dual objective is ``almost" strongly convex in the sense that it satisfies a strong-convexity condition with high-probability for all pairs of points sufficiently far apart.  
	\item With high-probability, the dual solution and the dual solution to the perturbed problem of the Danskin Correction are close for all $k$.   
\end{enumerate}

We show that the dual objective function satisfies a strong convexity property with high probability.  This argument relies on a covering that satisfies a certain set of properties. We show how to construct such  a covering in the following lemma.

\begin{lemma}\label[lem]{lem:cover-existance}
There exists a covering $\overline{\Lambda}$ on the set 
\[
\Lambda = \left \{ (\blambda_1, \blambda_2) \in \R^{2m} : \| \blambda_1 \|_1 \leq \lambda_{\max} \ \text{and} \  \| \blambda_2 \|_1 \leq \lambda_{\max} \ \text{and} \  
\left \Vert \blambda_1 - \blambda_2 \right \Vert_2 \ge \frac{4}{n}
\right\}.
\]
with the following properties:

i) For every $(\blambda_1, \blambda_2) \in \Lambda$ there exists $(\blambdabar_1,\blambdabar_2) \in \overline{\Lambda}$ such that $\left\Vert \blambdabar_i-\blambda_i \right\Vert _{2} \le 1/n$ for $ i=1,2$. 

ii) $\abs{\overline{\Lambda}} \le \left( 3n\lambda_{\max} \right)^{2m}$
\end{lemma}
\proof{Proof of \cref{lem:cover-existance}}
To construct an appropriate covering,  \cite{pollard1990empirical} states that the there exists a $1/n$-covering of
\[ 
	 \mathcal{L} =  \left \{ \blambda \in \R^{m} : \| \blambda \|_1 \leq \lambda_{\max}   \right\}.
\]
of size at most $(3n\lambda_{\max})^m$. Taking a cartesian-product of this covering with itself gives us a covering of $\Lambda$ satisfying i). We see ii) follows immediately.

\hfill \Halmos \endproof

With our covering we now state the specific strong-convexity property of our dual objective.

\begin{theorem}[Approximate Strong-Convexity of the Dual] \label[lem]{lem:StrongConvexity}
Fix any $\epsilon < 1/e$ and let $C_A>1$ and $\lambda_{\max} > e$.  Then,  there exists an $C$ (depending on $\lambda_{\max}$, $\phi_{\max}$, $C_A$) such that with probability at least $1-4\epsilon$, 
\begin{align}\
\frac{1}{n}\sum_{j=1}^{n}\mathbb{I}\left\{ Z_{j}\in\left\langle \bm{A}_{j}^{\top} \blambda_{1},\bm{A}_{j}^{\top}\blambda_{2}\right\rangle \right\} & \left|\bm{A}_{j}^{\top}\left(\blambda_1-\blambda_2\right)\right| \notag
 \\
\ge 
& \underbrace{
		\frac{\phi_{\min}{\beta}}{2}\left\Vert \blambda_1-\blambda_2\right\Vert _{2}^{2}
	}_{\text{Expected Strong Convexity}} 
	- 
\underbrace{C \cdot m \cdot  \log(n) \cdot \log\left(\frac{1}{\epsilon}\right)
			\frac{\left\Vert \blambda_1- \blambda_2\right\Vert _{2}^{3/2}}{\sqrt{n}}
	}_{\text{Uniform Error and Discretization Error }}
\end{align}
holds for all $\blambda_1, \blambda_2 \in \Lambda$.
\end{theorem}
%
%\begin{remark} \label{rmk:cover-construction}
%For the Theorem to work,  we ensure that a $O(1/n)$ covering exists where the elements in the covering are $1/n$ apart in $\ell_2$.  To construct the covering,  we construct a $1/n$ grid for each dimension of the $m-$dimensional dual solutions. For ``neighboring" components (for $\blambda_1,\blambda_2$ to be neighbors $\abs{\lambda_{1i}-\lambda_{2i}} \le 1/n$ for all $i=1,\dots,m$) of in the covering, the maximum $\ell_2$ distance is $\sqrt{m}/n$ while the minimum $\ell_2$ distance is $1/n$ (differing by one component).  This suggests we need to consider a $\sqrt{m}/n$ covering in order to guarantee the minimum distance condition. 
%\end{remark}
\subsection{Proof of \cref{lem:StrongConvexity}}
To develop intuition, note all subgradients of the dual objective function are of the form 
\[
\bm{b} - \frac{1}{n} \sum_{j=1}^n \I{ Z_j > \bA_j^\top \blambda } \bA_j - \frac{1}{n} \sum_{j=1}^n \I{Z_j = \bA_j^\top \blambda } \bA_j x_j,
\]
for some $x_j \in [0, 1]$.  At $\blambda(\bZ)$, the second term is $O_p(m/n)$, and, hence, negligible.  It follows that the analogue of the left side of \cref{eq:StrongConvexityDefinition} is 
\[
\frac{1}{n} \sum_{j=1}^n \left( \I{ Z_j > \bA_j^\top \blambda_2 }  - \I{ Z_j > \bA_j^\top \blambda_1 } \right) \bA_j^\top (\blambda_1 - \blambda_2) 
\ = \ 
\frac{1}{n} \sum_{j=1}^n \I{ Z_j  \in \langle \bA_j^\top \blambda_1, \bA_j^\top \blambda_2 \rangle  } \abs{ \bA_j^\top (\blambda_1 - \blambda_2) },
\]
where we have used our notation above to simplify.  Comparing \cref{eq:StrongConvexityDefinition} and \cref{lem:StrongConvexity}, we see that, intuitively, \cref{lem:StrongConvexity}  asserts that dual objective satisfies a condition quite close to strong-convexity for all points in $\Lambda$ not just $\overline{\Lambda}$.  

%Importantly, each summand is non-negative.  (Intuitively, the dual objective is convex and the sum is essentially the monotone gradient characterization of convexity.)

We prove \cref{lem:StrongConvexity} in several steps.  First we establish a similar result pointwise for a fixed $\blambda_1, \blambda_2$.  For convenience in what follows, define $X_j(\blambda_1, \blambda_2) \equiv \I{ Z_j \in \langle \bA_j^\top \blambda_1, \bA_j^\top \blambda_2 \rangle } \abs{ \bA_j ^\top (\blambda_1 - \blambda_2) }$.

\begin{lemma}[Pointwise Bound on Strong Convexity] \label[lem]{lem:pointwise}
Fix any $(\blambda_1, \blambda_2) \in  \R^{2m}$.  Then,  there exists a $C$ (depending on $\lambda_{\max},\phi_{\max},C_A$) such that with probability at least $1-\epsilon$, 
\[
\frac{1}{n} \sum_{j=1}^n X_j(\lambda_1, \lambda_2)
 \ \geq  \ 
\phi_{\min} \beta \| \blambda_1 - \blambda_2 \|_2^2 - C \cdot \sqrt{\frac{\log(1/\epsilon)}{n}} \| \blambda_1 - \blambda_2 \|^{3/2}.
\]
\end{lemma}
\proof{Proof of \cref{lem:pointwise}.}
  Compute 
\begin{align*}
\E{X_j(\blambda_1, \blambda_2) } 
	& = \abs{\bA_j^\top (\blambda_1 - \blambda_2) } \P{ Z_j \in \langle \bA_j \blambda_1, \bA_j \blambda_2 \rangle } 
\\ 
	& \geq \phi_{\min} \abs{\bA_j^\top (\blambda_1 - \blambda_2) }^2
\\
	& = \phi_{\min} \cdot (\blambda_1 - \blambda_2)^\top \bA_j \bA_j^\top (\blambda_1 - \blambda_2),
\end{align*}
where the inequality follows from \cref{asn:BoundedDensity}.  Similarly, 
\begin{align*}
\E{X_j(\blambda_1, \blambda_2)^2} 
	& \leq (\bA_j^\top (\blambda_1 - \blambda_2))^2 \cdot \P{ Z_j \in \langle \bA_j \blambda_1, \bA_j \blambda_2 \rangle }
\\
	& \leq 
\phi_{\max} \cdot (\bA_j^\top (\blambda_1 - \blambda_2))^3
\\ 
	& \leq
\phi_{\max}  C_A^3  \| \blambda_1 - \blambda_2 \|^3
\end{align*}
where the last line follows from \cref{asn:BoundedDensity}.

Furthermore, $X_j \geq 0$ almost surely.  Hence, by Eq. (2.23) of Wainright's book we have that 
\begin{align*}
\frac{1}{n} \sum_{j=1}^n X_j(\blambda_1, \blambda_2)  
	& \geq 
	\frac{1}{n} \sum_{j=1}^n \E{X_j (\blambda_1, \blambda_2)} - 
	\sqrt{ \frac{2 \log(1/\epsilon)}{n} } \sqrt{ \frac{1}{n} \sum_{j=1}^n \E{X_j(\lambda_1, \lambda_2)^2} }
\\
& \geq 
	\phi_{\min} (\blambda_1 - \blambda_2)^\top \frac{1}{n} \sum_{j=1}^n \bA_j \bA_j^\top (\blambda_1 - \blambda_2) 
	- \sqrt{ \frac{2 \log(1/\epsilon)}{n} } \sqrt{ \phi_{\max} } C_A^{3/2} \| \blambda_1 - \blambda_2\|^{3/2},
\\
& \geq 
	\phi_{\min} \beta \| \blambda_1 - \blambda_2 \|^2 - \sqrt{ \frac{2 \log(1/\epsilon)}{n} } \sqrt{ \phi_{\max} } C_A^{3/2} \| \blambda_1 - \blambda_2\|^{3/2},
\end{align*}
where the second inequality follows by substituting the bounds above and the third inequality follows from our assumption on the eigenvalues of $\frac{1}{n} \sum_{j=1}^n \bA_j \bA_j^\top$.  Rearranging proves the result.

\hfill \Halmos \endproof

Inspired by this pointwise result, we prove our uniform result (relative to a covering) by simply applying a covering of $\blambda$ and applying a union bound.  We simply apply a union bound over a covering satisfies the properties of \cref{lem:cover-existance}.  Since the covering for $\abs{ \Lambda }$ grows only polynomially in $n$,  we can extend our pointwise result to the covering.  
\begin{lemma}[Approximate Strong Convexity over the Covering]  \label[lem]{lem:ConvexityOnCovering}

Fix any $\epsilon < \frac{1}{e}$ and any $n > 3$.  Then, with probability at least $1-\epsilon$, 
\begin{align*}
\frac{1}{n} \sum_{j=1}^n X_j(\blambdabar_1, \blambdabar_2)
\ \geq  \ 
\phi_{\min} \beta \| \blambdabar_1 - \blambdabar_2 \|_2^2 - 2 \sqrt{ \phi_{\max} C_A^3 \log(3 \lambda_{\max} ) } \cdot \sqrt{\frac{m \log(1/\epsilon) \log(n)}{n}} \| \blambdabar_1 - \blambdabar_2 \|^{3/2} \\
\qquad \forall(\blambdabar_1, \blambdabar_2) \in \overline{\Lambda} 
.
\end{align*}
\end{lemma}
\proof{Proof of \cref{lem:ConvexityOnCovering}.}
From \cref{lem:cover-existance},
\[
\log\left( \frac{\abs{ \overline \Lambda } }{ \epsilon} \right)
 \ \leq \ 
2m \log \left( 3 n \lambda_{\max}  \right) + \log \left( \frac{1}{\epsilon}\right) \le
2m \log(3 \lambda_{\max} ) \log \left( \frac{1}{\epsilon}\right)  \log(n), 
\]
where the second inequality follows from our assumptions on the parameters.  Combining \cref{lem:pointwise} with a union bound then proves the result.  
\hfill \Halmos \endproof

Next, in anticipation of our discretization argument,  let $(\blambda_1, \blambda_2) \in \Lambda$ and let $(\blambdabar_1, \blambdabar_2) \in \overline \Lambda$ be the corresponding members of the covering such that $\| \blambda_i - \blambdabar_i \| \leq \frac{1}{n}$ for $ i = 1, 2$.  Then, 
we will ultimately need to upper bound 
\(
\frac{1}{n} \sum_{j=1}^n X_j(\blambdabar_1, \blambdabar_2) - X_j(\blambda_1, \blambda_2).
\)
We state the upper bound in the following lemma.
\begin{lemma}\label[lem]{lem:SimplifyingXdiff3}
For a $1/n-$covering $\overline{\Lambda}$,  the following holds for every $\blambda_1,\blambda_2 \in \Lambda$,
 \begin{align} \label{eq:SimplifyingXdiff3}
X_j(\blambdabar_1, \blambdabar_2) & - X_j(\blambda_1, \blambda_2) \\ \notag
	 \leq &
		C_A \| \blambdabar_1 - \blambdabar_2\| \left( \I{\abs{Z_j- \bA_j^\top \blambdabar_1} \leq  C_A / n} + \I{\abs{Z_j- \bA_j^\top \blambdabar_2} \leq  C_A / n} \right)
\\ \notag
& \quad + 
	 \frac{2 C_A}{n} \I{ \min( \bA_j^\top \blambdabar_1, \bA_j^\top \blambdabar_2 )  -  C_A / n \leq Z_j \leq \max( \bA_j^\top \blambdabar_1, \bA_j^\top \blambdabar_2 )  +  C_A / n } 
\end{align}
\end{lemma}
\proof{Proof of \cref{lem:SimplifyingXdiff3}.}
Write
\begin{align}  \label{eq:SimplifyingXdiff}
X_j(\blambdabar_1, \blambdabar_2) - X_j(\blambda_1, \blambda_2)
	 & = 
	\abs{\bA_j^\top(\blambdabar_1 - \blambdabar_2) } \left( \I{Z_j \in \langle \bA_j^\top \blambdabar_1, \bA_j^\top \blambdabar_2 \rangle} - \I{Z_j \in \langle \bA_j^\top \blambda_1, \bA_j^\top \blambda_2 \rangle} \right) 
\\ \notag
& \quad + 
	\left( \abs{\bA_j^\top(\blambdabar_1 - \blambdabar_2) } - \abs{\bA_j^\top(\blambda_1 - \blambda_2)} \right) \I{Z_j \in \langle \bA_j^\top \blambda_1, \bA_j^\top \blambda_2 \rangle} 
\end{align}
We simplify this expression.  Write
\begin{align*}
& \I{Z_j \in \langle \bA_j^\top \blambdabar_1, \bA_j^\top \blambdabar_2 \rangle} - \I{Z_j \in \langle \bA_j^\top \blambda_1, \bA_j^\top \blambda_2 \rangle}  
\\
 &\quad  = \abs{ \I{Z_j > \bA_j^\top \blambdabar_1} - \I{Z_j > \bA_j^\top \blambdabar_2} } 
 	- \abs{ \I{Z_j > \bA_j^\top \blambda_1} - \I{Z_j > \bA_j^\top \blambda_2} } 
\\
& \quad \leq \abs{ \I{Z_j > \bA_j^\top \blambdabar_1}  - \I{Z_j > \bA_j^\top \blambda_1} + \I{Z_j > \bA_j^\top \blambda_2} - \I{Z_j > \bA_j^\top \blambdabar_2} } 
		&&(\text{since } \abs{a} - \abs{b} \leq \abs{a-b})
\\
& \quad \leq 
\abs{ \I{Z_j > \bA_j^\top \blambdabar_1}  - \I{Z_j > \bA_j^\top \blambda_1} }  + \abs{ \I{Z_j > \bA_j^\top \blambda_2} - \I{Z_j > \bA_j^\top \blambdabar_2} }  
		&&(\text{by triangle inequality})
\\
& \quad = 
\I{Z_j \in \langle \bA_j^\top \blambdabar_1,  \bA_j^\top \blambda_1 \rangle} + 
\I{Z_j \in \langle \bA_j^\top \blambdabar_2,  \bA_j^\top \blambda_2 \rangle}				
\end{align*}
We now use the fact that $\| \blambda_i - \blambdabar_i \| \leq \frac{1}{n}$ for $i =1, 2$.  Indeed, 
\begin{align*}
\min(\bA_j^\top \blambdabar_i, \bA_j^\top \blambda_i) &\geq \bA_j^\top \blambdabar_i - C_A / n, 
\\
\max(\bA_j^\top \blambdabar_i, \bA_j^\top \blambda_i) &\leq \bA_j^\top \blambdabar_i + C_A / n,
\end{align*}
whereby
\(
\I{Z_j \in \langle \bA_j^\top \blambdabar_i,  \bA_j^\top \blambda_i \rangle} \leq \I{\abs{Z_j- \bA_j^\top \blambdabar_i} \leq C_A / n}.
\)  Substituting into \cref{eq:SimplifyingXdiff} yields, 
\begin{align} \label{eq:SimplifyingXdiff2}
X_j(\blambdabar_1, \blambdabar_2) & - X_j(\blambda_1, \blambda_2) \\ \notag
	 & = 
	C_A \| \blambdabar_1 - \blambdabar_2\|  \left( \I{\abs{Z_j- \bA_j^\top \blambdabar_1} \leq  C_A / n} + \I{\abs{Z_j- \bA_j^\top \blambdabar_2} \leq  C_A / n} \right)
\\ \notag
& \quad + 
	\left( \abs{\bA_j^\top(\blambdabar_1 - \blambdabar_2) } - \abs{\bA_j^\top(\blambda_1 - \blambda_2)} \right) \I{Z_j \in \langle \bA_j^\top \blambda_1, \bA_j^\top \blambda_2 \rangle} 
\end{align}

We can further simplify the second summand.  Specifically, 
\[
\abs{\bA_j^\top(\blambdabar_1 - \blambdabar_2) } - \abs{\bA_j^\top(\blambda_1 - \blambda_2)}  
\ \leq \ 
\abs{ \bA_j^\top(\blambdabar_1 - \blambda_1) + \bA_j (\blambda_2 - \blambdabar_2) }
\ \leq \ 
\abs{ \bA_j^\top(\blambdabar_1 - \blambda_1)} + \abs{\bA_j (\blambda_2 - \blambdabar_2) } 
\ \leq \ 
2  C_A / n.
\]
Moreover, 
\[
\I{ Z_j \in \langle \bA_j^\top \blambda_1, \bA_j^\top \blambda_2 \rangle } 
\  \leq \ 
\I{ \min( \bA_j^\top \blambdabar_1, \bA_j^\top \blambdabar_2 )  -  C_A / n \leq Z_j \leq \max( \bA_j^\top \blambdabar_1, \bA_j^\top \blambdabar_2 )  +  C_A / n }.
\]
Combining and substituting into \cref{eq:SimplifyingXdiff2} gives us our intended bound. 
\hfill \Halmos \endproof

It follows that if we want to bound the discretization error induced by our covering, we need to bound the right side of \cref{eq:SimplifyingXdiff3} uniformly over $\overline \Lambda$.  Although one might use a simple Hoeffding bound for both terms, the resulting rate is not fast enough.  The issue is that as $n \rightarrow \infty$ each indicator approaches $0$, and hence has small variance.

Consequently, we require the following (loose) bound on the sum of Bernoulli random variables:
\begin{lemma}[A Loose Bernstein Bound] \label[lem]{lem:LooseBernstein}
Suppose $Y_j \sim \text{Bernoulli}(p_j)$, independently across $j$, and $\frac{1}{n} \sum_{j=1}^n p_j \leq \overline p$.   Then, with probability at least $1-\epsilon$, 
\[
\frac{1}{n} \sum_{j=1}^n Y_j \leq \overline p + \frac{3 \log(1/\epsilon)}{n} \cdot \max\left( 1/3, \sqrt{ \overline p n} \right).
\]
\end{lemma}
\begin{remark}  A tighter analysis (in $\epsilon$) is possible using Bennet's inequality, but will not matter below.  The importance of the lemma is that it shows for $\overline p = O(1/n)$, the average is $\tilde O(1/n)$ rather than $\tilde O(1/\sqrt n)$ which is what arises from Hoeffding.
\end{remark}
\proof{Proof of \cref{lem:LooseBernstein}}
From Eq. 2.23 of Wainright's book,
\[
\P{ \frac{1}{n} \sum_{j=1}^n \left( Y_j - \E{Y_j} \right) > t } 
\ \leq \ 
	\exp\left(  \frac{-n t^2/2 }{ \frac{1}{n} \sum_{j=1}^n \E{Y_j^2} + t/3 }\right) 
\ \leq \ 
	\exp\left(  \frac{-n t^2/2 }{ \overline p + t/3 }\right), 
\]
where the second inequality uses $\E{Y_j^2} = \E{Y_j}$ and the definition of $\overline p$.  
Setting the right side equal to $\epsilon$ and rearranging yields
\begin{align} \label{eq:quadratic-exp}
	t^2 - \frac{2 \log(1/\epsilon)}{3n} t - \frac{2 \overline p \log(1/\epsilon)}{n} \geq 0.
\end{align}
Setting $\beta = \frac{2 \log(1/\epsilon)}{3n}$ and $\gamma = \frac{2 \overline p \log(1/\epsilon)}{n}$,  we see the quadratic function on the LHS has two real roots: $\frac{\beta \pm \sqrt{\beta^2 - 4\gamma}}{2}$.  Therefore, $t^2 - \beta t - \gamma \ge 0$ if and only if $t \le \frac{\beta - \sqrt{\beta^2 - 4\gamma}}{2}$ or $t \ge \frac{\beta + \sqrt{\beta^2 - 4\gamma}}{2}$. We upper bound the positive root of the quadratic equation as follows:
\begin{align*}
	\frac{\beta + \sqrt{\beta^2 + 4\gamma}}{2} \le \frac{\sqrt{2 (\beta^2 + \beta^2 - 4\gamma})}{2} = \sqrt{\beta^2 + 2 \gamma} 
\end{align*}
where the inequality follows from the fact that $\sqrt{x} + \sqrt{y} \le \sqrt{2(x + y)}$ for all $x,y \ge 0 $. 
Substituting back in $\beta$ and $\gamma$, we can see that \cref{eq:quadratic-exp} holds if
\[
t^2 
\ \leq \ 
	\frac{4}{9n^2 }  \log^2(1/\epsilon) + \frac{4 \overline p}{n} \log(1/\epsilon) 
\ \leq \ 
	\frac{4 \log^2 (1/\epsilon)}{n^2} \left( \frac{1}{9} + \overline p n \right)
\ \leq \ 
	\frac{8 \log^2 (1/\epsilon)}{n^2} \max\left( \frac{1}{9}, \overline p n \right).
\]
Taking the square root of both sides and noting $\sqrt{8} < 3$ proves the result.
\hfill \Halmos \endproof

We next use \cref{lem:LooseBernstein} to bound the indicators  \cref{eq:SimplifyingXdiff3}.

\begin{lemma} \label[lem]{lem:FirstTermDiscretization}
Fix any $\epsilon < \frac{1}{e}$ and any $n \geq 3$.  Assume $2 \phi_{\max} C_A > \frac{1}{9}$.  Then, there exists $C$ (depending on $C_A,\phi_{\max},\lambda_{\max}$) such that with probability at least $1-2\epsilon$, 
\begin{align*}
&	C_A \| \blambdabar_1 - \blambdabar_2\| \cdot \frac{1}{n} \sum_{j=1}^n \left( \I{\abs{Z_j- \bA_j^\top \blambdabar_1} \leq  C_A / n} + \I{\abs{Z_j- \bA_j^\top \blambdabar_2} \leq  C_A / n} \right)
\\ \quad & 
\ \leq \ 
 C_1 \cdot m \cdot \log(1/\epsilon)  \log(n)
\frac{\| \blambdabar_1 - \blambdabar_2 \|}{n}  
\end{align*}
holds simultaneously for all $(\blambdabar_1, \blambdabar_2) \in \overline{\Lambda}$, where $ \overline {\Lambda}$ is a $1/n-$cover of $\Lambda$.
\end{lemma}  
\proof{Proof of \cref{lem:FirstTermDiscretization}.}
If $\blambdabar_1 = \blambdabar_2$,  then the result trivially holds since both sides of the inequality are 0.

We now consider the case where $\blambdabar_1 \ne \blambdabar_2$.
First consider a fixed $(\blambdabar_1, \blambdabar_2) \in \overline \Lambda$.  We bound
\[
\frac{1}{n} \sum_{j=1}^n \P{\abs{Z_j- \bA_j^\top \blambdabar_i} \leq  C_A / n}
\ \leq \ 
C / n, \quad i = 1, 2. 
\]
where $C = 2 \phi_{\max}  C_A$. 
Then,  applying \cref{lem:LooseBernstein} once for each indicator yields the following upper-bound
\begin{align*}
&C_A \| \blambdabar_1 - \blambdabar_2\| \cdot  \frac{1}{n} \sum_{j=1}^n  \left( \I{\abs{Z_j- \bA_j^\top \blambdabar_1} \leq  C_A / n} + \I{\abs{Z_j- \bA_j^\top \blambdabar_2} \leq  C_A / n} \right)
\\  & \qquad
\ \leq \ 
2 C_A\cdot C \cdot \frac{\| \blambdabar_1 - \blambdabar_2 \|}{n}  + 
	6 C_A \sqrt{C}  \cdot  \log(1/\epsilon)    \frac{\| \blambdabar_1 - \blambdabar_2 \|}{n}
\\ & \qquad 
\ \leq \
C' \log(1/\epsilon)
\frac{\| \blambdabar_1 - \blambdabar_2 \|}{n}
\end{align*}
and the last inequality holds for $C' = 8\cdot C \cdot C_A$.

We now apply union bound letting $\epsilon \rightarrow  \epsilon / \abs{\overline \Lambda}$.  Recalling that 
\[
\log\left( \frac{\abs{ \overline \Lambda } }{ \epsilon} \right)
 \ \leq \ 
2m \log(3 \lambda_{\max} ) \log(1/\epsilon)  \log(n), 
\]
from \cref{lem:cover-existance},  rearranging, and letting $C_1 = 2 C'  \log(3 \lambda_{\max})$ proves the result. 
\hfill \Halmos \endproof

The second term in \cref{eq:SimplifyingXdiff3} is similar:
\begin{lemma} \label[lem]{lem:SecondTermDiscretization}
Fix any $\epsilon < \frac{1}{e}$, $n > 3$.  Assume $ 2 C_A \phi_{\max} > \frac{1}{9}$.  Then, there exists $C$ (depending on $C_A,\phi_{\max},\lambda_{\max}$) such that with probability at least $1-\epsilon$, 
\begin{align*}
& \frac{2 C_A}{n} \cdot  \frac{1}{n} \sum_{j=1}^n \I{ \min( \bA_j^\top \blambdabar_1, \bA_j^\top \blambdabar_2 )  -  C_A\sqrt{m} / n \leq Z_j \leq \max( \bA_j^\top \blambdabar_1, \bA_j^\top \blambdabar_2 )  +  C_A\sqrt{m} / n } 
\\
\quad  \leq  &
	 C_1 \cdot m \cdot \log (1/e)  \log(n) 
	 \left( 
		\frac{1}{n^2} +
		\frac{\| \blambdabar_1 - \blambdabar_2 \|}{n}  +
		\frac{\| \blambdabar_1 - \blambdabar_2 \|^{3/2}}{\sqrt{n}} 
	\right)
\end{align*}
holds simultaneously for all $(\blambdabar_1, \blambdabar_2) \in \overline{\Lambda}$, where $ \overline {\Lambda}$ is a $1/n-$cover of $\Lambda$.
\end{lemma}
\proof{Proof of \cref{lem:SecondTermDiscretization}.}
If $\blambdabar_1 = \blambdabar_2$,  then the result holds since the indicators are 0 almost surely.  Thus,  both sides of the inequality are 0.

We now consider the case where $\blambdabar_1 \ne \blambdabar_2$.
First, we bound 
\begin{align*}
&\P{ \min( \bA_j^\top \blambdabar_1, \bA_j^\top \blambdabar_2 )  -  C_A / n \leq Z_j \leq \max( \bA_j^\top \blambdabar_1, \bA_j^\top \blambdabar_2 )  +  C_A / n }
\\ & \quad  \ \leq \ 
 \phi_{\max} (2  C_A / n + C_A \| \blambdabar_1 - \blambdabar_2 \|) 
\\ & \quad \ \leq \ 
 C \left( \frac{1}{n} + \| \blambdabar_1 - \blambdabar_2\|  \right)
 \end{align*}
 where $C = 2 C_A \phi_{\max}$. 
 Hence, by \cref{lem:LooseBernstein}, for any fixed $(\blambdabar_1, \blambdabar_2) \in \overline \Lambda$ such that $\blambdabar_1 \ne \blambdabar_2$,   we have
 \begin{align*}
& 2  C_A / n \cdot  \frac{1}{n} \sum_{j=1}^n \I{ \min( \bA_j^\top \blambdabar_1, \bA_j^\top \blambdabar_2 )  -  C_A / n  \leq Z_j \leq \max( \bA_j^\top \blambdabar_1, \bA_j^\top \blambdabar_2 )  +  C_A / n } 
\\
&\quad  \leq 
 \frac{2 C_A }{ n } \cdot \left(  
	  C \left( \frac{1}{n} + \| \blambdabar_1 - \blambdabar_2 \| \right) + 
	  \frac{3\log(1/\epsilon ) }{n} \sqrt{ C \cdot n \cdot \left( \frac{1}{n} + \| \blambdabar_1 - \blambdabar_2 \| \right) } 
 \right) 
 \\
& \quad \leq 
	  \frac{2C\dot C_A + 6\sqrt{C} C_A \log (1/e)}{n^2} + 
	  2 C \cdot C_A \frac{ \| \blambdabar_1 - \blambdabar_2 \|}{n} + 
	  6 \log(1/\epsilon )C_A \sqrt{C} \cdot \frac{\| \blambdabar_1 - \blambdabar_2 \|^{3/2}}{\sqrt{n}} 
\\
& \quad \leq 
	C' \log (1/e) \left( 
		\frac{1}{n^2} +
		\frac{\| \blambdabar_1 - \blambdabar_2 \|}{n}  +
		\frac{\| \blambdabar_1 - \blambdabar_2 \|^{3/2}}{\sqrt{n}} 
	\right)
\end{align*}
where the last line let $C' = 8 C \cdot C_A$.
Applying the union bound after noting
\[
\log\left( \frac{\abs{ \overline \Lambda } }{ \epsilon} \right)
 \ \leq \ 
2m 	\log(3 \lambda_{\max}) \log(1/\epsilon)  \log(n), 
\]
from \cref{lem:cover-existance}, rearranging, and letting \[C_1= 2 C' \log (3 \lambda_{\max}),\] we obtain the intended bound.
\hfill \Halmos \endproof

We now prove \cref{lem:StrongConvexity}.
\proof{Proof of \cref{lem:StrongConvexity}.}
Without loss of generality,  we consider the case where $2 \phi_{\max} C_A > \frac{1}{9}$ (if not we can scale $C_A$ up for the strict inequality to be true).
Recall 
\[X_j(\blambda_1, \blambda_2) \equiv \I{ Z_j \in \langle \bA_j^\top \blambda_1, \bA_j^\top \blambda_2 \rangle } \abs{\bA_j^\top(\blambda_1 - \blambda_2) }.\]
   Choose any $(\blambda_1, \blambda_2) \in \Lambda$ and let $(\blambdabar_1, \blambdabar_2) \in \overline \Lambda$ be the corresponding members of the covering such that $\| \blambda_i - \blambdabar_i \| < \sqrt{m}/n$ for $i = 1, 2$.  Then, with probability at least $1-\epsilon$, 
\begin{align*}
\frac{1}{n} \sum_{j=1}^n X_j(\blambda_1, \blambda_2) 
& = 
\frac{1}{n} \sum_{j=1}^n X_j(\blambdabar_1, \blambdabar_2)  - 
\frac{1}{n} \sum_{j=1}^n \left( X_j(\blambdabar_1, \blambdabar_2) - X_j(\blambda_1, \blambda_2) \right)
\\
& \geq \phi_{\min} \beta \| \blambdabar_1 - \blambdabar_2 \|_2^2 - C_1 \cdot \sqrt{\frac{m \log(1/\epsilon)  \log(n)}{n}} \| \blambdabar_1 - \blambdabar_2 \|^{3/2} 
\\
& \qquad - 
\frac{1}{n} \sum_{j=1}^n \left( X_j(\blambdabar_1, \blambdabar_2) - X_j(\blambda_1, \blambda_2) \right)
\\ 
& \geq \phi_{\min} \beta \| \blambdabar_1 - \blambdabar_2 \|_2^2 - C_1 \cdot \sqrt{\frac{m \log(1/\epsilon)  \log(n) }{n}} \| \blambdabar_1 - \blambdabar_2 \|^{3/2} 
\\ & \qquad 
	- C_A \| \blambdabar_1 - \blambdabar_2\| \frac{1}{n} \sum_{j=1}^n \left( \I{\abs{Z_j- \bA_j^\top \blambdabar_1} \leq  C_A\sqrt{m} / n} + \I{\abs{Z_j- \bA_j^\top \blambdabar_2} \leq  C_A\sqrt{m} / n} \right)
\\ \notag
& \qquad - 
	 \frac{2 C_A}{n} \I{ \min( \bA_j^\top \blambdabar_1, \bA_j^\top \blambdabar_2 )  -  C_A\sqrt{m} / n \leq Z_j \leq \max( \bA_j^\top \blambdabar_1, \bA_j^\top \blambdabar_2 )  +  C_A\sqrt{m} / n } 
 \end{align*}
where the first inequality follows from \cref{lem:ConvexityOnCovering} and the second from \cref{eq:SimplifyingXdiff3}.  We now apply \cref{lem:FirstTermDiscretization,lem:SecondTermDiscretization} to bound the above average.  Hence, with probability at least $1-4\epsilon$, 
\begin{align*}
\frac{1}{n} \sum_{j=1}^n X_j(\blambda_1, \blambda_2)  & \geq 
\phi_{\min} \beta \| \blambdabar_1 - \blambdabar_2 \|_2^2 - C_1 \cdot \sqrt{\frac{m \log(1/\epsilon)  \log(n)}{n}} \| \blambdabar_1 - \blambdabar_2 \|^{3/2} 
\\ & \qquad 
 - C_2 \cdot m \cdot \log(1/\epsilon)  \log(n)
\frac{\| \blambdabar_1 - \blambdabar_2 \|}{n}  
\\
& \qquad   - 
	C_3 \cdot m \cdot \log(1/\epsilon)  \log(n)
	\left( 
		\frac{1}{n^2} +
		\frac{\| \blambdabar_1 - \blambdabar_2 \|}{n}  +
		\frac{\| \blambdabar_1 - \blambdabar_2 \|^{3/2}}{\sqrt{n}} 
	\right)
\end{align*}
To convert the $\| \blambdabar_1 - \blambdabar_2 \|$ term to $\| \blambda_1 - \blambda_2 \|$, we see
\[
	\| \blambdabar_1 - \blambdabar_2 \| 
	\le 
	\| \blambda_1 - \blambda_2 \| + \frac{2}{n}
	\le 
	\frac{3}{2}\| \blambda_1 - \blambda_2 \|
\]
\[
	\| \blambdabar_1 - \blambdabar_2 \| 
	\ge 
	\| \blambda_1 - \blambda_2 \| - \frac{2}{n}
	\ge 
	\frac{1}{2}\| \blambda_1 - \blambda_2 \|
\]
where the first inequality for both lines follows triangle inequality and the second inequality for both lines follows our assumption that $\| \blambda_1 - \blambda_2 \| \ge \frac{4}{n}$.

Substituting and using the fact that $\frac{1}{2}\| \blambda_1 - \blambda_2 \|^{1/2} \ge \frac{1}{\sqrt{n}}$, we see
\begin{align*}
\frac{1}{n} \sum_{j=1}^n X_j(\blambda_1, \blambda_2)  & 
\geq 
\frac{\phi_{\min} \beta}{2} \| \blambda_1 - \blambda_2 \|_2^2 
- C_1 \left(\frac{3}{2}\right)^{3/2} \cdot \sqrt{\frac{m \log(1/\epsilon)  \log(n)}{n}} \| \blambda_1 - \blambda_2 \|^{3/2} 
\\ & \qquad 
 - C_2 \cdot \frac{3}{2} \cdot m \cdot \log(1/\epsilon)  \log(n)
\frac{\| \blambda_1 - \blambda_2 \|^{3/2}}{2\sqrt{n}} 
\\
& \qquad   - 
	C_3 \cdot \left(\frac{3}{2}\right)^{3/2} \cdot m \cdot \log(1/\epsilon)  \log(n)
	\left( 
		\frac{\| \blambda_1 - \blambda_2 \|^{3/2}}{2\sqrt{2}\sqrt{n}} +
		\frac{\| \blambda_1 - \blambda_2 \|^{3/2}}{2\sqrt{n}}  +
		\frac{\| \blambda_1 - \blambda_2 \|^{3/2}}{\sqrt{n}} 
	\right)
\end{align*}
Collecting the terms,  so that 
\[
 C = \left(\frac{3}{2}\right)^{3/2} C_1 
 + \frac{3}{4} C_2 
 + 3 \left(\frac{3}{2}\right)^{3/2} C_3 
 \le 408 C_A^2 \max(\phi_{\max},\sqrt{\phi_{\max}}) \log\left(3 \lambda_{\max} \right),
\]
we obtain our result.
\hfill \Halmos \endproof

\section{Proof of \cref{thm:dual-sol-bound}}
\label{sec:thm-3.1-proof}
We now show that the dual variables have a bounded distance for any two vectors 
$\bZ,\overline{\bZ} \in \mathcal{Y} (\epsilon)$, where
\[
	\mathcal{Y} (\epsilon)
	\equiv
	\left\{
		\bZ : \left\Vert \blambda(\bZ) \right\Vert _{1} \le \lambda_{\max} \text{ and \cref{eq:str-cvx-cond} is satisfied}
	\right\}
\]
\begin{theorem}
Let $\bZ,\overline{\bZ}\in \mathcal{Y}(\epsilon)$, then there exists $C$ (depending on $\lambda_{\max}$, $\phi_{\min}$, $\phi_{\max}$, $\beta$, $C_A$) such that 
\begin{align*}
	\left\Vert \blambda(\bZ) - \blambda(\overline{\bZ}) \right\Vert_2 \le 
	\frac{C m^2 \log^{2}n\log^{2}\left(\frac{1}{\epsilon}\right)}{n} 
	\sum_{j=1}^{n}	
	\mathbb{I}\left\{ Z_{j}\ne\bar{Z}_{j}\right\}
\end{align*}
\end{theorem}
\proof{Proof of \cref{thm:dual-sol-bound}}
Our argument leverages the convexity of the dual objectives. Let $f_{1}(\blambda)\equiv\bm{b}^{\top}\blambda+\frac{1}{n}\sum_{j=1}^{n}\left[Z_{j}-\bA_{j}^{\top}\blambda\right]^{+}$
and $f_{2}(\blambda)\equiv\bm{b}^{\top}\blambda+\frac{1}{n}\sum_{j=1}^{n}\left[\bar{Z}_{j}-\bA_{j}^{\top}\blambda\right]^{+}$.
Additionally, let $\blambda_{i}\in\arg\min_{\blambda\ge0}f_{i}(\blambda)$
so that $\blambda_{1}=\blambda(\bZ)$ and $\blambda_{1}=\blambda(\overline{\bZ})$.
Since $f_{i}(\blambda)$ are convex, we see that 
\begin{align}\label{eq:cvx-prop}
f_{1}(\blambda_{2})-f_{1}(\blambda_{1})\ge\nabla f_{1}(\blambda_{1})^{\top}(\blambda_{2}-\blambda_{1})
\end{align}
 where $\nabla$ denotes the sub-gradient. Additionally, we see that
\begin{align}\label{eq:cvx-opt-cond}
\nabla f_{1}\left(\blambda_{2}\right)^{\top}\left(\blambda_{1}-\blambda_{2}\right)\le f_{1}(\blambda_{1})-f_{1}(\blambda_{2})\le0
\end{align}
 by optimality. Thus,
\begin{align*}
f_{1}(\blambda_{2})-f_{1}(\blambda_{1}) & \ge\nabla f_{1}(\blambda_{1})^{\top}(\blambda_{2}-\blambda_{1}), \qquad \text{from \cref{eq:cvx-prop}}\\
 & \ge\nabla f_{1}(\blambda_{1})^{\top}(\blambda_{2}-\blambda_{1})+\nabla f_{1}\left(\blambda_{2}\right)^{\top}\left(\blambda_{1}-\blambda_{2}\right), \qquad \text{from \cref{eq:cvx-opt-cond}}\\
 & =\left[\nabla f_{1}\left(\blambda_{1}\right)-\nabla f_{1}\left(\blambda_{2}\right)\right]^{\top}(\blambda_{2}-\blambda_{1}).
\end{align*}
A similar argument can be made to show the same result, but with the
indices swapped,
\[
f_{2}(\blambda_{1})-f_{2}(\blambda_{2})\ge\left[\nabla f_{2}\left(\blambda_{2}\right)-\nabla f_{2}\left(\blambda_{1}\right)\right]^{\top}(\blambda_{1}-\blambda_{2}).
\]
Summing the two inequalities, we have
\begin{align}\label{eq:cvx-relation}
	f_{1}(\blambda_{2})-f_{1}(\blambda_{1})
	+
	f_{2}(\blambda_{1})-f_{2}(\blambda_{2})
	\ge \\ \notag
	\left[\nabla f_{1}\left(\blambda_{1}\right)-\nabla f_{1}\left(\blambda_{2}\right)\right]^{\top} & (\blambda_{2}-\blambda_{1})
	+
	\left[\nabla f_{2}\left(\blambda_{2}\right)-\nabla f_{2}\left(\blambda_{1}\right)\right]^{\top}(\blambda_{1}-\blambda_{2}).
\end{align}

Using this inequality, we construct an upper-bound of the left hand
side and a lower-bound of the right hand side by leveraging a Lipchitz
bound and a strong convexity bound, respectively. This will allow
us to bound our dual solution.

To bound the left hand side, first note that,
\begin{align*}
 & \left[f_{1}(\blambda_{2})-f_{1}(\blambda_{1})\right]+\left[f_{2}(\blambda_{1})-f_{2}(\blambda_{2})\right]\\
= & \frac{1}{n}
	\sum_{j=1}^{n}
	\left[Z_{j}-\bA_{j}^{\top}\blambda_{2}\right]^{+}
	- \left[Z_{j}-\bA_{j}^{\top}\blambda_{1}\right]^{+}
	+ \left[\overline{Z}_{j}-\bA_{j}^{\top}\blambda_{1}\right]^{+}
	- \left[\overline{Z}_{j}-\bA_{j}^{\top}\blambda_{2}\right]^{+}.
\end{align*}
We see that the $j^{\text{th}}$ component can be upper-bounded as follows,
\begin{align*}
 & \frac{1}{n}
	\sum_{j=1}^{n}
	\left[Z_{j}-\bA_{j}^{\top}\blambda_{2}\right]^{+}
	- \left[Z_{j}-\bA_{j}^{\top}\blambda_{1}\right]^{+}
	+ \left[\overline{Z}_{j}-\bA_{j}^{\top}\blambda_{1}\right]^{+}
	- \left[\overline{Z}_{j}-\bA_{j}^{\top}\blambda_{2}\right]^{+} \\
 \le &  
 \min
 \left\{
 	2\left|\bA_{j}^{\top}\blambda_{1}-\bA_{j}^{\top}\blambda_{2}\right|, 
 	2\left|Z_{j}-\bar{Z}_{j}\right|
 \right\} \\
 \le & 
  \min
 \left\{
 	2C_{A}\left\Vert \blambda_{1}-\blambda_{2}\right\Vert _{2},
 	2\left|Z_{j}-\bar{Z}_{j}\right|
 \right\} 
\end{align*}
where the first inequality comes from upper-bounding 
\(
	\left[Z_{j}-\bA_{j}^{\top}\blambda_{2}\right]^{+}
	- \left[Z_{j}-\bA_{j}^{\top}\blambda_{1}\right]^{+}
\)
for the first term in the minimum and 
\(
	\left[Z_{j}-\bA_{j}^{\top}\blambda_{i}\right]^{+}
	- \left[\overline{Z}-\bA_{j}^{\top}\blambda_{i}\right]^{+}
\)
for the second term in the minimum.
We further upper-bound the last line by combining the two terms in the minimum to show
\begin{align}\label{eq:upp-bound}
\left[f_{1}(\blambda_{2})-f_{2}(\blambda_{2})\right]+\left[f_{2}(\blambda_{1})-f_{1}(\blambda_{1})\right]
\le
\frac{1}{n}\sum_{j=1}^{n}2C_{A}\left\Vert \blambda_{1}-\blambda_{2}\right\Vert _{2}\mathbb{I}\left\{ Z_{j}\ne\bar{Z}_{j}\right\} 
\end{align}

To lower bound the right hand side relative to $\overline{\Lambda}$,  we see that the subgradient $\nabla f_i\left(\blambda_i \right)$
of the dual objective (wlog for $i=1$) can be written as 
\[
	\bm{b} + \frac{1}{n} \sum_{j=1}^{n} 
	\mathbb{I}\left\{ Z_{j} > \bm{A}_{j}^{\top}\blambda \right\} \bm{A}_{j}
	- \frac{1}{n}\sum_{j=1}^{n}\mathbb{I}\left\{ Z_{j} = \bm{A}_{j}^{\top}\blambda\right\} \bm{A}_{j}x_{j}\left(\bZ\right),
\]
where the last term follows from complementary slackness. We can lower
bound the right hand side of \cref{eq:cvx-relation} by first lower bounding the first term (the second term follows an identical argument)
as follows
\begin{align}\label{eq:subgrad-comp}
 & \left[
 	\nabla f_1\left(
 		\blambda_1
 	\right)
 	- \nabla f_1 \left(
 		\blambda_2
 	\right)
 	\right]^{\top}
 	\left(\blambda_2 -\blambda_1\right) \\ \notag
	= & \underbrace{
		\frac{1}{n} \sum_{j=1}^{n}
		\left(
			\mathbb{I}\left\{ Z_{j} > \bm{A}_{j}^{\top} \blambda_1 \right\} 
			- \mathbb{I}\left\{ Z_{j} > \bm{A}_{j}^{\top}\blambda_2 \right\} 
		\right)
		\bm{A}_{j}^{\top}\left(\blambda_2 - \blambda_1\right)
	}_{(a)} \\ \notag
 & \qquad - \underbrace{
 	\frac{1}{n} \sum_{j=1}^{n}
 	\left(\mathbb{I}\left\{ Z_{j} = \bm{A}_{j}^{\top}\blambda_1 \right\} x_{j}\left(\bZ\right)
 	- \mathbb{I}\left\{ Z_{j} = \bm{A}_{j}^{\top}\blambda_2 \right\}
 	x_{j}\left(\bZ\right)
 	\right)
 	\bm{A}_{j}^{\top}\left(\blambda_2 -\blambda_1 \right)}_{(b)}.
\end{align}
We first consider upper bounding the term $(b)$.  Thus,
\begin{align} \label{eq:up-bnd-b}
 &
 	\frac{1}{n}\sum_{j=1}^{n}
 	\left(
 		\mathbb{I}\left\{ Z_{j}=\bm{A}_{j}^{\top}\blambda_1 \right\} 
 		x_{j}\left(\bZ\right)
 		- \mathbb{I}\left\{ Z_{j} = \bm{A}_{j}^{\top}\blambda_2 \right\} 
 		x_{j}\left(\bZ\right)
 	\right) 
 	\bm{A}_{j}^{\top}\left(\blambda_2-\blambda_1\right)
 	\\ \notag
 	\le & \frac{1}{n}
 		\sum_{j=1}^{n}
 		\left|
 			\mathbb{I}\left\{ Z_{j}=\bm{A}_{j}^{\top}\blambda_1\right\} 
 			x_{j}\left(\bZ\right)
 			- \mathbb{I}\left\{ Z_{j}=\bm{A}_{j}^{\top}\blambda_2 \right\} 
 			x_{j}\left(\bZ\right)
 		\right|
 		\left| 
 		\bm{A}_{j}^{\top}\left(\blambda_2-\blambda_1\right)
 		\right| \\ \notag
	\le & \frac{1}{n} C_A
		\left\Vert \blambda_2 -\blambda_1 \right\Vert _{2} \sum^n_{j=1} \left|
 			\mathbb{I}\left\{ Z_{j}=\bm{A}_{j}^{\top}\blambda_1\right\} 
 			x_{j}\left(\bZ\right)
 			- \mathbb{I}\left\{ Z_{j}=\bm{A}_{j}^{\top}\blambda_2 \right\} 
 			x_{j}\left(\bZ\right)
 		\right| \\ \notag
	\le & \frac{C_{A}m}{\sqrt{n}}
	\left\Vert \blambda_2 - \blambda_1 \right\Vert _{2}^{3/2}
\end{align}
where the second inequality comes from upper-bounding 
$\left| \bm{A}_{j}^{\top}\left(\blambda_2-\blambda_1\right) \right|$ and the last inequality comes from noting that for a fixed $\bZ$, the indicators $\mathbb{I}\left\{ Z_{j}=\bm{A}_{j}^{\top}\blambda(\bZ)\right\} $
are non-zero for at most $m$ terms.  

To lower bound (a),  we rewrite the $j^{\text{th}}$
term of the summation as 
\[
\mathbb{I}\left\{ Z_{j}\in\left\langle \bm{A}_{j}^{\top}\blambda_1,\bm{A}_{j}^{\top}\blambda_2 \right\rangle \right\} \left|\bm{A}_{j}^{\top}\left(\blambda_2 - \blambda_1 \right)\right|
\]
Using \cref{eq:str-cvx-cond}, we see that for 
$\left\Vert \blambda_{2} - \blambda_{1}\right\Vert _{2} \ge \frac{4}{n}$,
\begin{align}\label{eq:lwr-bnd-a}
(a)
\ge
	\frac{\phi_{\min}{\beta}}{2}\left\Vert \blambda_{2}- \blambda_{1}\right\Vert _{2}^{2}
	- C \cdot m \cdot  \log(n) \cdot \log\left(\frac{1}{\epsilon}\right)
	\left(
			\frac{\left\Vert \blambda_{2} - \blambda_{1}\right\Vert _{2}^{3/2}}{\sqrt{n}}
	\right)
\end{align}

Thus, to prove the theorem,  we now consider two cases i) $\left\Vert \blambda_{2} - \blambda_{1}\right\Vert _{2} < \frac{4}{n}$ and ii) $\left\Vert \blambda_{2} - \blambda_{1}\right\Vert _{2} \ge \frac{4}{n}$.  

Case i) trivially satisfies the bound,  thus, we focus on case ii).

In case ii),  we combine our bounds on (a) (\cref{eq:lwr-bnd-a}) and (b) (\cref{eq:up-bnd-b}) and group terms to show the RHS of \cref{eq:cvx-relation}
is lower bounded by
\begin{align}\label{eq:rhs-bound}
	\phi_{\min}{\beta}\left\Vert \blambda_{2} - \blambda_{1}\right\Vert _{2}^{2}
	- 2 (C + C_A) \cdot m \cdot  \log(n) \cdot \log\left(\frac{1}{\epsilon}\right)
			\frac{\left\Vert \blambda_{2} - \blambda_{1}\right\Vert _{2}^{3/2}}{\sqrt{n}},
\end{align}
where the extra factor $2$ comes from lowering bounding the sum of the two terms. 
It then follows from the combining the upper-bound on the LHS (\cref{eq:upp-bound}) and the lower bound on the
RHS (\cref{eq:rhs-bound}) of \cref{eq:cvx-relation} and collecting dominant terms that
\begin{align}\label{eq:first-result}
	(4 C_{A} + 2C) \cdot m \cdot 
	\log(n) \cdot \log\left(\frac{1}{\epsilon}\right)
	\frac{\left\Vert \blambda_2 - \blambda_1 \right\Vert _{2}^{3/2}}{\sqrt{n}}
	\sum_{j=1}^{n}	
	\mathbb{I}\left\{ Z_{j}\ne\bar{Z}_{j}\right\}
& 
\ge
 \phi_{\min}{\beta}\left\Vert \blambda_2 - \blambda_1 \right\Vert _{2}^{2}
\end{align}

Dividing both sides by $\left\Vert \blambda_{2} - \blambda_{1}\right\Vert _{2}^{3/2}$,  we get
\begin{align}\label{eq:second-result}
 C_0 \cdot m \cdot  \log(n) \cdot \log\left(\frac{1}{\epsilon}\right)
\frac{1}{\sqrt{n}}
\sum_{j=1}^{n}	
	\mathbb{I}\left\{ Z_{j}\ne\bar{Z}_{j}\right\}
& 
\ge
\left\Vert \blambda_2 - \blambda_1 \right\Vert _{2}^{1/2}
\end{align}
where $C_0 \equiv \frac{(4 C_{A} + 2C)}{\phi_{\min}{\beta}}$.

Using \cref{eq:second-result} to substitute in for $\left\Vert \blambda_2 - \blambda_1 \right\Vert _{2}^{1/2}$,  we further lower-bound \cref{eq:rhs-bound} by,
\begin{align*}
	\phi_{\min}{\beta}\left\Vert \blambda_{2} - \blambda_{1}\right\Vert _{2}^{2}
	- 2C^2_0 \cdot m^{2} \cdot  \log^2(n) \cdot \log^2 \left(\frac{1}{\epsilon}\right)
			\frac{\left\Vert \blambda_{2} - \blambda_{1}\right\Vert _{2}}{n}
			\sum_{j=1}^{n}	
	\mathbb{I}\left\{ Z_{j}\ne\bar{Z}_{j}\right\}
\end{align*}
Combining this with the LHS upper-bound (\cref{eq:upp-bound}),  we get
\begin{align}
	(C_0 +C_0^2) \cdot m\cdot 
	\log^2 (n) \cdot \log^2 \left(\frac{1}{\epsilon}\right)
	\frac{\left\Vert \blambda_2 - \blambda_1 \right\Vert _{2}}{n}
	\sum_{j=1}^{n}	
	\mathbb{I}\left\{ Z_{j}\ne\bar{Z}_{j}\right\}
& 
\ge
 \phi_{\min}{\beta}\left\Vert \blambda_2 - \blambda_1 \right\Vert _{2}^{2}
\end{align}
Dividing both sides by 
$\left\Vert \blambda_{2} - \blambda_{1}\right\Vert _{2}$
we get 
\begin{align*}
	\frac{C_{1} m^2 \log^{2}n\log^{2}\left(\frac{1}{\epsilon}\right)}{n} 
	\sum_{j=1}^{n}	
& 
\ge
	\left\Vert \blambda_2 - \blambda_1 \right\Vert _{2}.
\end{align*}
where $C_1 = C_0 + C_0^2$.
\hfill \Halmos \endproof

\begin{corollary} \label{cor:stability-dual-sol-cor}
Let $\bZ\in\mathcal{Y}(\epsilon)$ and $\overline{\bZ}^k=\bZ + Y \be_k$ such that $\left \Vert \blambda(\overline{\bZ}) \right \Vert_1 \le \lambda_{\max}$.  Then,  there exists $C$ (depending on $\lambda_{\max}$, $\phi_{\min}$, $\phi_{\max}$, $\beta$, $C_A$) such that 
\begin{align*}
	\left\Vert \blambda(\bZ) - \blambda(\overline{\bZ}^k) \right\Vert_2 \le 
	\frac{C m^2 \log^{2}n\log^{2}\left(\frac{1}{\epsilon}\right)}{n} 
\end{align*}
\end{corollary}
\proof{Proof of \cref{cor:stability-dual-sol-cor}}
To prove the result in the case where $\overline{\bZ}^k$ potentially is not in the set $\mathcal{Y}(\epsilon)$, we only need construct a new lower bound for the (a) term for $\overline{\bZ}^k$,
\begin{align*}
	&
	\frac{1}{n} \sum_{j=1}^{n}
		\left(
			\mathbb{I}\left\{ \overline{Z}^k_{j} > \bm{A}_{j}^{\top} \blambda_1 \right\} 
			- \mathbb{I}\left\{ \overline{Z}^k_{j} > \bm{A}_{j}^{\top}\blambda_2 \right\} 
		\right)
		\bm{A}_{j}^{\top}\left(\blambda_2 - \blambda_1\right) \\
	\ = \
	& 
	\frac{1}{n} \sum_{j=1}^{n}
		\left(
			\mathbb{I}\left\{ Z_{j} \in \langle \bA_j^\top \blambda_1, \bA_j^\top \blambda_2 \rangle \right\}
		\right)
		\left| \bm{A}_{j}^{\top}\left(\blambda_2 - \blambda_1\right) \right| \\
	& \qquad + \frac{1}{n} \left(
			\mathbb{I}\left\{ Z_{k} + Y \in \langle \bA_j^\top \blambda_1, \bA_j^\top \blambda_2 \rangle \right\} 
			-
			\mathbb{I}\left\{ Z_{k} \in \langle \bA_j^\top \blambda_1, \bA_j^\top \blambda_2 \rangle \right\} 
		\right)
		\left| \bm{A}_{j}^{\top}\left(\blambda_2 - \blambda_1\right) \right| \\
	\ \ge \
	& \frac{\phi_{\min}{\beta}}{2}\left\Vert \blambda_{2}- \blambda_{1}\right\Vert _{2}^{2}
	- C \cdot m \cdot  \log(n) \cdot \log\left(\frac{1}{\epsilon}\right)
	\left(
			\frac{\left\Vert \blambda_{2} - \blambda_{1}\right\Vert _{2}^{3/2}}{\sqrt{n}}
	\right) 
	- C_A \frac{\left\Vert \blambda_{2} - \blambda_{1}\right\Vert _{2}^{3/2}}{2\sqrt{n}}.
\end{align*}
The first equality holds by writing the difference of indicators as one indicator and the second inequality comes from using the original lower bound of (a) and noting that
\[
	\left(
			\mathbb{I}\left\{ Z_{k} + Y \in \langle \bA_j^\top \blambda_1, \bA_j^\top \blambda_2 \rangle \right\} 
			-
			\mathbb{I}\left\{ Z_{k} \in \langle \bA_j^\top \blambda_1, \bA_j^\top \blambda_2 \rangle \right\} 
		\right)
		\left| \bm{A}_{j}^{\top}\left(\blambda_2 - \blambda_1\right) \right| \le C_A \frac{\left\Vert \blambda_{2} - \blambda_{1}\right\Vert _{2}}{n}
\]
as well as $\frac{1}{2}\left\Vert \blambda_{2} - \blambda_{1}\right\Vert _{2}^{1/2} \ge \frac{1}{\sqrt{n}}$. This only changes the constant $C$ of the original lower bound on (a) by a constant $C_A$. Hence, we obtain the same result. 
\hfill \Halmos \endproof
